# Supplementary material for: Global-Local Self-Distillation for Visual Representation Learning
Source: arXiv:2207.14676 source file (2022-10-12)
Supplement: Supplementary file 1 [file appendix_global-local.tex]

% \begin{figure*}[t]
%   \centering
%   %\fbox{\rule{0pt}{2in} \rule{0.9\linewidth}{0pt}}
%   \includegraphics[width=0.96\textwidth]{fig/all_local.png}

%   \caption{\textbf{Visualization of our inverse distance-based weighted local-representation matching between 2 augmentations (1 global-crop and 1 local-crop) of an input image.} Each location on a coarse grained grid (corresponding to the area of an output token) on the right view is linked to the best matching location on the left view based on the distance between the center of the locations w.r.t. the original input image (left). The width of the matching lines corresponds to the weighting which is computed relative to all other matching distances. The smaller the matching distance is in the input image, the higher the weighting is. Colors are used only to better differentiate different matchings.}
%   \label{fig:global-local}
% \end{figure*}

% \afterpage{%
% \thispagestyle{plain}
\begin{figure*}[p]
\centering
\includegraphics[width=0.96\textwidth]{fig/all_local.png}
\caption{\textbf{Visualization of our inverse distance-based weighted local-representation matching between 2 augmentations (1 global-crop and 1 local-crop) of an input image.} Each location on a coarse grained grid (corresponding to the area of an output token) on the right view is linked to the best matching location on the left view based on the distance between the center of the locations w.r.t. the original input image (left). The width of the matching lines corresponds to the weighting which is computed relative to all other matching distances. The smaller the matching distance is in the input image, the higher the weighting is. Colors are used only to better differentiate different matchings.}
\label{fig:global-local}
\end{figure*}
% \clearpage
% }
